# Supplementary material for: InstantStyle: Free Lunch towards Style-Preserving in Text-to-Image Generation
Source: arXiv:2404.02733 source file (2024-04-04)
Supplement: Supplementary file 1 [file Appendix.tex]

\newpage

\section{Supplementary Details}

\subsection{Implementation Detail}

In Figure~\ref{fig:editbility}, the spatial control, canny image (b) and depth image (c) are extracted from a same reference pose image Figure~\ref{fig:supp1} (a).

\begin{figure}[htbp]
  \centering
  \vspace{-0.3cm}
  \includegraphics[width=0.7\textwidth]{Figures/supp1.pdf}
  \caption{The spatial controls extracted from a reference image.}
  \label{fig:supp1}
  \vspace{-0.5cm}
\end{figure}

\subsection{Supplementary Results}

\begin{figure}[htbp]
  \centering
  \vspace{-0.6cm}
  \includegraphics[width=0.7\textwidth]{Figures/param-xy.pdf}
  \caption{\textbf{Effect of Image Adapter and IdentityNet.} The x-axis and y-axis correspond to the weight strength of Image Adapter and IdentityNet respectively.}
  \label{fig:param-xy}
  \vspace{-0.5cm}
\end{figure}

\begin{figure}[htbp]
  \centering
  \includegraphics[width=\textwidth]{Figures/novel-view.pdf}
  \caption{\textbf{Novel View Synthesis under any given pose.}}
  \label{fig:novel-view}
  % \vspace{0.1cm}
\end{figure}

\begin{figure}[htbp]
  \centering
  \includegraphics[width=\textwidth]{Figures/id-interpolation.pdf}
  \caption{\textbf{Identity interpolation between different characters.}}
  \label{fig:id-interpolation}
  % \vspace{0.1cm}
\end{figure}

\begin{figure}[htbp]
  \centering
  \includegraphics[width=\textwidth]{Figures/multiid.pdf}
  \caption{\textbf{Multi-identity synthesis with regional control.}}
  \label{fig:multiid}
\end{figure}
